# Supplementary material for: Approximate Minimum Diameter
Source: arXiv:1703.10976 source file (2017-03-31)
Supplement: Supplementary file 1 [file appendix.tex]

\subsection{Reducing the number of constraints}\label{const}

In this section, we describe how to reduce the number of constraints in $LP$~\ref{LP1}. For this, we use Observation \ref{triv}. 

\begin{obs}
$|x|$ is the smallest value $z$ such that $z \geq x$ and $z \geq -x$. 
\label{triv}
\end{obs}

Thus, for the following $LP$, we have $z = |x|$:
\begin{equation}
\label{LP2}
\begin{array}{ll@{}ll}
\textbf{LP~\ref{LP2}:}  & &\\
\text{minimize}  &\quad \displaystyle  z &\\
\text{subject to}&\quad \displaystyle x \ &\leq z  &\quad\\
                 &\displaystyle -x &\leq z &\quad
\end{array}
\end{equation}

We use Observation~\ref{triv} to modify $LP$~\ref{LP1} into $LP$~\ref{LP3}. In $LP$~\ref{LP3}, $Q$ is a large enough integer, ensuring that minimizing $\ell$ is more important than $\sum d_{i,j,k}$. 

\begin{equation}
\label{LP3}
\begin{array}{ll@{}ll}
\textbf{LP~\ref{LP3}:}  & &\\
\text{minimize}  &\quad \displaystyle  Q\ell\ + \sum d_{i,j,k} & &\\

\text{subject to}&\quad \displaystyle \sum_k d_{i,j,k}  \leq \ell &\quad\forall i,j\\
&\quad \displaystyle  s_{i} \in {\cal R}_i &\quad\forall i,j\\
&\quad \displaystyle d_{i,j,k} \geq s_{i,k} - s_{j,k} &\quad\forall i,j,k\\
&\quad \displaystyle d_{i,j,k} \geq s_{j,k} - s_{i,k} &\quad\forall i,j,k

\end{array}
\end{equation}

Number of the constraints in $LP$~\ref{LP3} is $O(n^2 d + |{\cal R}|)$ which is $\textsf{poly}(n)$.
